# Supplementary material for: TF-DCon: Leveraging Large Language Models (LLMs) to Empower Training-Free Dataset Condensation for Content-Based Recommendation
Source: arXiv:2310.09874 source file (2025-02-09)
Supplement: Supplementary file 1 [file Appendix.tex]

\clearpage
\appendix
\section{{Algorithm for EvoPro}}
\label{sec:appendix}
\input{sections/sub-sections/Algorithm-EvoPro}
\section{{Algorithm for TF-DCon}}
\input{sections/sub-sections/Algorithm-TF-DCon}
